# Supplementary material for: Statistical Model and Estimation Method for Ranging a Moving Ship Using a Single Acoustic Receiver in Shallow Water
Source: arXiv:2505.01562 source file (2025-08-27)
Supplement: Supplementary file 1 [file SuppPub1.pdf]

# THEORETICAL JUSTIFICATION AND DERIVATION OF THE STATISTICAL PARAMETER ESTIMATORS

This document provides a detailed probabilistic justification and derivation of the estimators required to compute the proposed likelihood function. The signal models are considered in the striation-frequency domain representation of the acoustic intensities. Striations and frequencies are indexed by  $l \in \mathcal{L}$  and  $k \in \mathcal{K}$ , respectively. The total number of frequency bins is  $K = |\mathcal{K}|$ . The subset of frequencies containing only broadband components of ship-radiated noise is denoted by  $\mathcal{K}^b$ , while the subset containing both tonal and broadband components denote by  $\mathcal{K}^{bt}$ . There are  $J$  bins in  $\mathcal{K}^{bt}$ .

For  $k \in \mathcal{K}^b$ , the intensity follows an exponential distribution, i.e.,

$$\underline{x}_{l,k}^b \sim \text{Exp}(\underline{x}_{l,k}^b; \underline{\theta}_{l,k} = \underline{\sigma}_{l,k}^2)$$

where  $\underline{\theta}_{l,k}$  is the scaling factor. In the main manuscript, the scaling factor was shown to have the same value as the broadband-plus-noise variance  $\underline{\sigma}_{l,k}^2$ . For  $k \in \mathcal{K}^{bt}$ , the normalized intensity follows a noncentral- $\chi^2$  distribution, i.e.,

$$\underline{y}_{l,k}^{bt} \sim \chi^2(\underline{y}_{l,k}^{bt}; d = 2, \underline{\lambda}_{l,k})$$

where  $d = 2$  is the degrees of freedom, and  $\underline{\lambda}_{l,k}$  is the noncentrality parameter. We assume that intensities are statistically independent across striations and frequencies. For additional notation and signal model details, see Sec. III of the main manuscript.

To obtain the maximum likelihood estimate (ML) of the ship's range, we estimate the scaling factor  $\underline{\theta}_{l,k}$  and the noncentrality parameter  $\underline{\lambda}_{l,k}$  using Kolmogorov's Strong Law of Large Numbers (SLLN).

## I. BACKGROUND

To estimate the statistical parameters governing the probability density functions (PDFs) of the intensities and normalized intensities, we employ the Strong Law of Large Numbers (SLLN) and Kolmogorov's criterion<sup>1</sup>. Specifically, Kolmogorov's SLLN states that if  $\{X_n\}$  is a sequence of mutually independent random variables with common distribution and finite mean  $\mathbb{E}[X_n] = \mu$ , then the sample mean converges almost surely to  $\mu$ , i.e.,

$$\frac{1}{N} \sum_{n=1}^N X_n \xrightarrow{\text{a.s.}} \mu \text{ as } n \rightarrow \infty. \quad (1)$$

Kolmogorov's criterion extends this result to sequences of mutually independent but not necessarily identically distributed random variables. If  $X_n$  has finite mean  $\mathbb{E}[X_n] = \mu_n$  and variance  $\sigma_n^2 = \text{Var}(X_n)$ , and if the sequence satisfies

$$\sum_{n=1}^{\infty} \frac{\sigma_n^2}{n^2} < \infty$$

then the SLLN holds in the extended form, i.e.,

$$\frac{1}{N} \sum_{n=1}^N X_n \xrightarrow{\text{a.s.}} \frac{1}{N} \sum_{n=1}^N \mu_n \text{ as } N \rightarrow \infty. \quad (2)$$

In the application considered in this paper, we can assume that the variance of the intensities,  $\underline{x}_{l,k}^b$ , is bounded across both striations and frequencies. This assumption is supported by (i) the behavior of the channel transfer function, whose magnitude decays with range due to modal attenuation and spreading losses in a shallow water waveguide<sup>2</sup>, and (ii) the finite energy of the ship's radiated noise and the presence of a constant (finite) background noise variance.

## II. BROADBAND-PLUS-NOISE VARIANCE ESTIMATION

To compute the normalized intensities, we estimate the broadband-plus-noise variance  $\underline{\sigma}_{l,k}^2$ . As shown in the main manuscript, the broadband-plus-noise variance  $\underline{\sigma}_{l,k}^2$  is equal to the scaling factor  $\underline{\theta}_{l,k}$ . Based on Eq. (19) in the main manuscript, we can write

$$\underline{\theta}_{l,k} = (\sigma_k^b |g_{l,k}|)^2 + (\sigma_k^u)^2.$$

Note that the background noise  $(\sigma_k^u)^2$  is assumed known. For a given frequency index  $k \in \mathcal{K}^b$ , we defined  $\eta_k = \sigma_k^b / \sigma_{k'}^b$  ( $\eta_k > 0$ ) as the ratio of broadband signal standard deviations at  $f_k$  and a reference frequency  $f_{k'}$ , where  $k' \in \mathcal{K}^b$  is arbitrarily chosen. Based on the frequency-dependent Green's function relation  $|g_{l,k}| = \gamma_k |g_{l,k'}|$  as presented in Eq. (11) of the main manuscript, we obtain

$$\underline{\theta}_{l,k} = (\eta_k \gamma_k)^2 (\sigma_{k'}^b |g_{l,k'}|)^2 + (\sigma_k^u)^2. \quad (3)$$

We define the received broadband scale parameter  $\alpha_k = (\eta_k \gamma_k)^2$  and the received broadband signal variance  $\underline{v}_{l,k} = (\sigma_k^b)^2 |g_{l,k}|^2$ . By using these definitions of  $\alpha_k$  and  $\underline{v}_{l,k}$  in Eq. (3), as well as flipping the terms on the right-hand side, we obtain

$$\underline{\theta}_{l,k} = (\sigma_k^u)^2 + \alpha_k \underline{v}_{l,k}. \quad (4)$$

Next, we compute an estimate of  $\underline{\theta}_{l,k}$ , by separately computing estimates of  $\alpha_k$  and  $\underline{v}_{l,k}$ .

### A. Broadband Scale Parameter $\alpha_k$

Since  $\mathbb{E}[\underline{x}_{l,k}^b] = \underline{\theta}_{l,k}$ , applying the SLLN with Kolmogorov's criterion in Eq. (2), the sample mean satisfies

$$\frac{1}{L} \sum_{l \in \mathcal{L}} \underline{x}_{l,k}^b \xrightarrow{\text{a.s.}} \frac{1}{L} \sum_{l \in \mathcal{L}} \underline{\theta}_{l,k}. \quad (5)$$

Let us average the scaling factor  $\underline{\theta}_{l,k}$  across striations (cf. Eq. (4)), i.e.,

$$\frac{1}{L} \sum_{l \in \mathcal{L}} \underline{\theta}_{l,k} = (\sigma_k^u)^2 + \alpha_k \frac{1}{L} \sum_{l \in \mathcal{L}} \underline{v}_{l,k}. \quad (6)$$

For a sufficiently large number of striations, we can make

use of Eq. (5) such that, after rearranging Eq. (6) for  $\alpha_k$ , we obtain

$$\alpha_k = \frac{\frac{1}{L} \sum_{l \in \mathcal{L}} \underline{x}_{l,k}^b - (\sigma_k^u)^2}{\frac{1}{L} \sum_{l \in \mathcal{L}} \underline{v}_{l,k'}}.$$

Since  $\alpha_{k'} = 1$  at the reference frequency  $f_{k'}$ , for the frequency index  $k = k'$ , the average in Eq. (6) reads

$$\frac{1}{L} \sum_{l \in \mathcal{L}} \underline{v}_{l,k'} = \frac{1}{L} \sum_{l \in \mathcal{L}} \underline{x}_{l,k'}^b - (\sigma_{k'}^u)^2.$$

By substituting the denominator of Eq. (7) with the relationship in Eq. (7), an estimate of the broadband scale parameter is obtained as

$$\hat{\alpha}_k = \frac{\frac{1}{L} \sum_{l \in \mathcal{L}} \underline{x}_{l,k}^b - (\sigma_k^u)^2}{\frac{1}{L} \sum_{l \in \mathcal{L}} \underline{x}_{l,k'}^b - (\sigma_{k'}^u)^2}. \quad (7)$$

### B. Received Broadband Signal Variance $\underline{v}_{l,k}$

The broadband signal variance is estimated using a similar approach. Assuming independence across frequency bins and bounded variance, the sample mean at striation index  $l \in \mathcal{L}$  converges, i.e.,

$$\frac{1}{K-J} \sum_{k \in \mathcal{K}^b} \underline{x}_{l,k}^b \xrightarrow{\text{a.s.}} \frac{1}{K-J} \sum_{k \in \mathcal{K}^b} \underline{\theta}_{l,k}. \quad (8)$$

Next, we average the scaling factor  $\underline{\theta}_{l,k}$  across frequencies (cf. Eq. (4)), i.e.,

$$\frac{1}{K-J} \sum_{k \in \mathcal{K}^b} \underline{\theta}_{l,k} = (\sigma_k^u)^2 + \underline{v}_{l,k'} \frac{1}{K-J} \sum_{k \in \mathcal{K}^b} \alpha_k. \quad (9)$$

For a sufficiently large number of measurements across frequencies, we can use Eq. (8) in Eq. (9), i.e.,

$$\frac{1}{K-J} \sum_{k \in \mathcal{K}^b} \underline{x}_{l,k}^b = (\sigma_k^u)^2 + \underline{v}_{l,k'} \frac{1}{K-J} \sum_{k \in \mathcal{K}^b} \alpha_k.$$

After solving this expression for  $\underline{v}_{l,k'}$ , we obtain

$$\underline{v}_{l,k'} = \frac{1}{\sum_{k \in \mathcal{K}^b} \alpha_k} \left( \sum_{k \in \mathcal{K}^b} \underline{x}_{l,k}^b - (\sigma_k^u)^2 \right). \quad (10)$$

By substituting the broadband scale parameter  $\alpha_k$  in Eq. (10) with its estimate  $\hat{\alpha}_k$  in Eq. (7), an estimate of the received broadband-plus-noise variance is finally calculated as

$$\hat{\underline{v}}_{l,k'} = \frac{1}{\sum_{k \in \mathcal{K}^b} \hat{\alpha}_k} \left( \sum_{k \in \mathcal{K}^b} \underline{x}_{l,k}^b - (\sigma_k^u)^2 \right). \quad (11)$$

### C. Broadband-plus-noise Variance $\underline{\sigma}_{l,k}^2$

Based on Eqs. (4), (7) and (11), an estimate of  $\underline{\theta}_{l,k}$  is obtained as

$$\hat{\underline{\theta}}_{l,k} = \hat{\alpha}_k \hat{\underline{v}}_{l,k'} + (\sigma_k^u)^2.$$

Finally, the estimate of the broadband-plus-noise variance  $\underline{\sigma}_{l,k}^2$ , is given by  $\hat{\underline{\sigma}}_{l,k}^2 = \hat{\underline{\theta}}_{l,k}$ , with  $\hat{\underline{\theta}}_{l,k}$  as presented in Eq. (18) of the main manuscript. In our practical implementation, we set  $\hat{\underline{\sigma}}_{l,k}^2 = 0$  in case  $\hat{\underline{\sigma}}_{l,k}^2$  is negative. We also apply a moving average filter to  $\hat{\underline{\sigma}}_{l,k}^2$  across striations at each frequency. This helps to reduce the variance of the estimated parameters, leading to an improved overall performance.

## III. NONCENTRALITY PARAMETER ESTIMATION

We estimate the noncentrality parameter  $\underline{\lambda}_{l,k}$  for the normalized intensity  $\underline{y}_{l,k}^{\text{bt}}$  at striation  $l \in \mathcal{L}$  and frequency index  $k \in \mathcal{K}^{\text{bt}}$ . The expectation of  $\underline{y}_{l,k}^{\text{bt}}$  is denoted by  $\underline{\mu}_{l,k}^{\text{bt}} = \mathbb{E}[\underline{y}_{l,k}^{\text{bt}}]$  and expressed as

$$\underline{\mu}_{l,k}^{\text{bt}} = d + \underline{\lambda}_{l,k} \quad (12)$$

where  $d = 2$  is the degrees of freedom<sup>3</sup>. Following the model in Sec. IV C 2 of the main manuscript, we assume that  $\underline{\lambda}_{l,k}$  can be expressed as a product of a striation-dependent parameter and a frequency-dependent scaling factor,

$$\underline{\lambda}_{l,k} = \underline{\lambda}_l \rho_k \quad (13)$$

where  $\rho_k > 0$  is a frequency-dependent scale factor, and  $\underline{\lambda}_l$  is the striation-wise noncentrality parameter.

For clarity in the derivation below, we use  $i$  and  $j$  instead of  $l$  and  $k$  when summing over striations and frequencies, respectively. This helps distinguish the indices being summed over from the particular index of interest, denoted as  $(l, k)$ .

Assuming that the normalized intensities satisfy Kolmogorov's criterion, the sample mean across striations at fixed frequency index  $k$  converges to the corresponding expected mean, i.e.,

$$\frac{1}{L} \sum_{i \in \mathcal{L}} \underline{y}_{i,k}^{\text{bt}} \xrightarrow{\text{a.s.}} \frac{1}{L} \sum_{i \in \mathcal{L}} \underline{\mu}_{i,k}^{\text{bt}}. \quad (14)$$

Similarly, at a fixed striation index  $l$ , the sample mean across frequencies converges to the expected average, i.e.,

$$\frac{1}{J} \sum_{j \in \mathcal{K}^{\text{bt}}} \underline{y}_{l,j}^{\text{bt}} \xrightarrow{\text{a.s.}} \frac{1}{J} \sum_{j \in \mathcal{K}^{\text{bt}}} \underline{\mu}_{l,j}^{\text{bt}}. \quad (15)$$

Furthermore, by using Eq. (13) in Eq. (12), and by averaging  $\underline{\mu}_{l,k}^{\text{bt}}$  over striations at fixed frequency  $k$  leads to

$$\frac{1}{L} \sum_{i \in \mathcal{L}} \underline{\mu}_{i,k}^{\text{bt}} = 2 + \rho_k \frac{1}{L} \sum_{i \in \mathcal{L}} \underline{\lambda}_i \quad (16)$$

while averaging  $\underline{\mu}^{\text{bt}}$  over frequencies at fixed striation  $l$  results in

$$\frac{1}{J} \sum_{j \in \mathcal{K}^{\text{bt}}} \underline{\mu}_{l,j}^{\text{bt}} = 2 + \underline{\lambda}_l \frac{1}{J} \sum_{j \in \mathcal{K}^{\text{bt}}} \rho_j. \quad (17)$$

For a sufficiently large number of measurements across striations and across frequencies, we can apply Eqs. (14) and (15) to Eqs. (16) and (17), respectively. In this way, we obtain

$$\frac{1}{L} \sum_{i \in \mathcal{L}} \underline{y}_{i,k}^{\text{bt}} = 2 + \rho_k \frac{1}{L} \sum_{i \in \mathcal{L}} \underline{\lambda}_i$$

and

$$\frac{1}{J} \sum_{j \in \mathcal{K}^{\text{bt}}} \underline{y}_{l,j}^{\text{bt}} = 2 + \underline{\lambda}_l \frac{1}{J} \sum_{j \in \mathcal{K}^{\text{bt}}} \rho_j.$$

Similarly, the full average of the normalized intensities across all striations and frequencies is given by

$$\begin{aligned} \frac{1}{JL} \sum_{j \in \mathcal{K}^{\text{bt}}} \sum_{i \in \mathcal{L}} \underline{y}_{i,j}^{\text{bt}} &= d + \frac{1}{JL} \sum_{j \in \mathcal{K}^{\text{bt}}} \sum_{i \in \mathcal{L}} \underline{\lambda}_i \rho_j \\ &= 2 + \frac{1}{JL} \sum_{i \in \mathcal{L}} \underline{\lambda}_i \sum_{j \in \mathcal{K}^{\text{bt}}} \rho_j. \end{aligned} \quad (18)$$

By rearranging Eqs. (16) and (17), we obtain

$$\rho_k = \frac{\frac{1}{L} \sum_{i \in \mathcal{L}} \underline{y}_{i,k}^{\text{bt}} - 2}{\frac{1}{L} \sum_{i \in \mathcal{L}} \underline{\lambda}_i} \quad (19)$$

$$\underline{\lambda}_l = \frac{\frac{1}{J} \sum_{j \in \mathcal{K}^{\text{bt}}} \underline{y}_{l,j}^{\text{bt}} - 2}{\frac{1}{J} \sum_{j \in \mathcal{K}^{\text{bt}}} \rho_j}. \quad (20)$$

Substituting Eqs. (19) and (20) into Eq. (18) yields

$$\underline{\lambda}_{l,k} = \frac{\left( \frac{1}{J} \left( \sum_{j \in \mathcal{K}^{\text{bt}}} \underline{y}_{l,j}^{\text{bt}} \right) - 2 \right) \left( \frac{1}{L} \left( \sum_{i \in \mathcal{L}} \underline{y}_{i,k}^{\text{bt}} \right) - 2 \right)}{\frac{1}{JL} \left( \sum_{i \in \mathcal{L}} \underline{\lambda}_i \right) \left( \sum_{j \in \mathcal{K}^{\text{bt}}} \rho_j \right)}. \quad (21)$$

Note that the denominator of the above equation is still a function of unknown variables  $\rho_j$  and  $\lambda_i$ . To address this, we first rearrange Eq. (18) as follows

$$\frac{1}{JL} \sum_{i \in \mathcal{L}} \underline{\lambda}_i \sum_{j \in \mathcal{K}^{\text{bt}}} \rho_j = \frac{1}{JL} \sum_{j \in \mathcal{K}^{\text{bt}}} \sum_{i \in \mathcal{L}} \underline{y}_{i,j}^{\text{bt}} - 2. \quad (22)$$

Next, we replace the denominator of Eq. (21), by the right hand side of Eq. (22). In this way, we obtain the following estimate of the noncentrality parameter

$$\hat{\underline{\lambda}}_{l,k} = \frac{\left( \frac{1}{J} \left( \sum_{j \in \mathcal{K}^{\text{bt}}} \underline{y}_{l,j}^{\text{bt}} \right) - 2 \right) \left( \frac{1}{L} \left( \sum_{i \in \mathcal{L}} \underline{y}_{i,k}^{\text{bt}} \right) - 2 \right)}{\frac{1}{JL} \sum_{j \in \mathcal{K}^{\text{bt}}} \sum_{i \in \mathcal{L}} \underline{y}_{i,j}^{\text{bt}} - 2}$$

also is presented in Eq. (27) in Sec. IV B of the main manuscript.

At low SNR, the subtraction by two may be negative, and the denominator may be numerically unstable. Thus, when its value is negative or unrealistically large, the noncentrality parameter is set to zero, i.e.,  $\hat{\underline{\lambda}}_{l,k} = 0$ . In addition, a moving average is applied to the noncentrality parameter along the striation axis at each frequency.

<sup>1</sup>W. Feller, *An introduction to probability theory and its applications*, Chap. 10.7 (Wiley, New York).

<sup>2</sup>F. B. Jensen, W. A. Kuperman, M. B. Porter, and H. Schmidt, in *Computational Ocean Acoustics*, 2nd ed. (Springer Publishing Company, Incorporated, 2011), Chap. 2.4 and 5.14.

<sup>3</sup>M. Evans, N. Hastings, and B. Peacock, in *Statistical distributions*, 3rd ed. (John Wiley & Sons, 2000), Chap. 9.
