# Supplementary material for: Statistical Model and Estimation Method for Ranging a Moving Ship Using a Single Acoustic Receiver in Shallow Water
Source: arXiv:2505.01562 source file (2025-08-27)
Supplement: Supplementary file 2 [file SuppPub2.pdf]

This supplementary document provides a detailed analysis of the waveguide invariant (WI). We obtained the WI value of  $\beta = 1.18$  at the beginning of the considered event (18:58-19:10 UTC, March 24th, 2017, during SBCEX17) for the 42–49 Hz frequency band. This value is higher than the commonly expected value of  $\beta \approx 1$  in a shallow-water environment with an isovelocity sound speed profile (SSP) and relatively uniform bathymetry<sup>1</sup>. One possible factor contributing to this deviation is variability in the geoacoustic properties of the seabed<sup>2,3</sup>, for which detailed information was not available at long ranges in the considered event.

The mode-pairwise waveguide invariant (WI), denoted  $\beta_{mn}$ , was introduced by Rouseff and Spindel<sup>4</sup>. While the scalar WI  $\beta$  summarizes the overall interference structure as a single parameter,  $\beta_{mn}$  characterizes the interference contribution from a specific mode pair  $m$  and  $n$  (see Sec. I A of the main manuscript). This mode-pairwise perspective is particularly useful in low-frequency bands where only a few modes propagate<sup>5</sup>. In our case, the 75 m water depth and a shortest wavelength of approximately 30 m (based on an SSP of 1470 m/s at 49 Hz) suggest that only a few modes are supported—especially at longer distances where higher-order modes attenuate. We therefore focus on estimating  $\beta_{mn}$  for the dominant mode pair as an independent validation of the scalar WI value ( $\beta = 1.18$ ) used in the main manuscript.

## I. METHOD

We perform two analyses based on the method proposed by Le Gall and Bonnel<sup>5</sup>. First, we apply the method to a shorter spectrogram (10 minutes) to examine the evolution of propagating mode pairs over time and range. This analysis reveals that only a single dominant mode pair persists beyond 19:02, corresponding to a source-receiver range of 19.5 km at the final snapshot of the spectrogram. The spectrogram time indicates the time associated with this final snapshot. In the second analysis, we estimate the waveguide invariant for this dominant mode pair using a longer spectrogram (47 minutes). Since this mode pair is the only source of observable modal interference at long distances, its WI value effectively characterizes the environment, justifying the use of a single scalar WI. To support this estimation, we utilize relative dispersion curves (RDCs)<sup>5</sup>, which graphically represent the frequency-dependent difference in horizontal wavenumbers between mode pairs. RDCs provide a useful visualization of modal contributions, particularly in environments where only a few modes propagate, allowing us to assess the consistency and structure of interference patterns over range and frequency.

## A. Extracting Modal Contributions using RDCs

We first normalize the range-frequency ( $r$ - $f$ ) surface plot by multiplying each snapshot by its corresponding range to compensate for geometric spreading effects<sup>5</sup>. The ranges here are computed from the geo-locations reported by the container ship via Automated Identification System (AIS). Then, to identify the modal contributions to the interference pattern, we perform a discrete Fourier transform (DFT) along the range axis at each frequency in the spectrogram. This transformation shifts the representation from range to the horizontal wavenumber  $k$  domain, where peaks correspond to dominant modal interactions. Since mode pairs exhibit interference at characteristic wavenumber differences, the x-axis of the resulting RDC plots is labeled as the wavenumber difference  $\Delta k$ . The summary of the operation is as follows:

$$\tilde{I}(\Delta k, f) = DFT_r[r \cdot I(r, f)], \quad (1)$$

where  $DFT_r[\cdot]$  denotes the DFT operation along the range-axis and  $I(r, f)$  represents the received acoustic intensity function at the corresponding range-frequency coordinates. Each energy peak in the  $\Delta k$  domain corresponds to the influence of a specific mode pair, and the RDC curve represents the trend of these energy peaks across frequency.

## B. Estimating Mode-Pairwise WI ( $\beta_{mn}$ )

To compute the waveguide invariant  $\beta_{mn}$  for the mode pair  $m$  and  $n$ , we inspect the RDCs in the logarithmic domain of the variables  $\Delta k$  and  $f$ , where the slope of each RDC satisfy the following relationship<sup>5</sup>:

$$\log(\Delta k_{mn}(f)) = \frac{-1}{\beta_{mn}} \cdot \log(f) + \log(\alpha_{mn}), \quad (2)$$

where  $\alpha_{mn}$  is a mode-dependent constant. This equation reveals that the slope of the RDC in the log-log domain is directly related to the WI of the mode pair  $\beta_{mn}$ . In practice, before interpolating in the log-log domain, we also normalized  $\tilde{I}(\Delta k, f)$  at each frequency by its frequency-wise maximum. The normalization reduces the bias introduced due to the frequency-wise variation of the intensities due to the ship radiated sound signature, leading to a more accurate slope estimation of these RDC curves.

To estimate  $\beta_{mn}$ , we apply the Radon transform to the RDCs in the log-log domain of  $\Delta k$  and  $f$ . The Radon transform integrates function values along straight lines at different angles, effectively identifying the dominant slope corresponding to each mode pair's WI. In this context, the angle of integration lines relative to the coordinate axes corresponds to the slope of the RDCs. The line that maximizes the Radon transform output is used to determine the WI. The best-aligned line with the observed RDC yields the highest integration response, and its angle is used to compute the slope (i.e.,  $-1/\beta_{mn}$ ) in

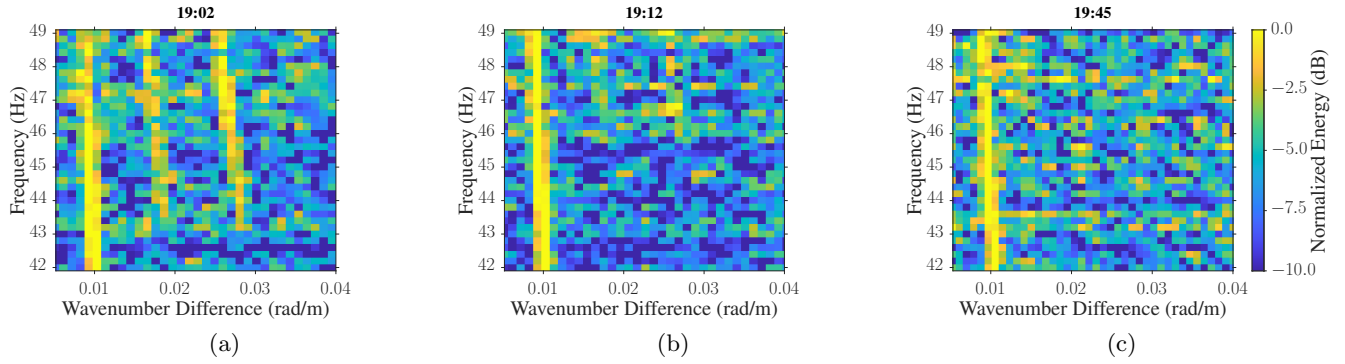

FIG. 1. Relative dispersion curves (RDCs) derived from acoustic recordings during the ship's transit relative to VLA 2 at three different times. They are obtained from performing Eq. 1 from the spectrograms. (a) The  $\tilde{I}(\Delta k, f)$  plot computed from the spectrogram from acoustic data recorded between 18:53 and 19:02, corresponding to ranges from 13.5 to 19.5 km. Prominent vertical lines correspond to the RDCs of mode pairs 12, 13, and 23 (from left to right). Since the geoacoustic properties of the environment at greater distances from VLA 2 are not fully characterized, the mode pairs are labeled arbitrarily as 12, 13, and 23, in order of increasing  $\Delta k$ . For (b) and (c), The plots of  $\tilde{I}(\Delta k, f)$  were obtained from the spectrogram from 19:03 to 19:12 (covering ranges of 19.5–25.6 km) and the spectrogram from 19:36 to 19:45 (covering ranges of 32.3–45.6 km), respectively. By the time of the spectrogram shown in (b), the mode pairs 13 and 23 have completely faded, leaving only mode pair 12.

Eq. (2)). This process ensures that the dominant WI value per mode pair is extracted systematically.

This approach offers a detailed characterization of the WI per pair of modes compared to assuming a single constant value. Specifically, it reveals how individual mode pairs shape the observed interference structure and contribute to WI variability, particularly in environments and frequency bands where only a few modes propagate.

## II. RESULTS AND DISCUSSION

**RDCs and Mode Pair Evolution:** The RDC curves shown in Fig. 1 correspond to the vertical bands of high intensities in the  $\Delta k$  and  $f$  domain. In Fig. 1 (a), the spectrogram corresponding to the earliest time interval (18:53 - 19:02) reveals three distinct vertical RDC curves, confirming the presence of three propagating modes at the beginning of the scenario. These three modes form three mode pairs, although the specific pairing order is not known. We designate the leftmost curve as the interference between mode pair 1 and 2, as the other two curves disappear over time, due to the attenuation of the third mode. For brevity, we adopt the shorthand notation “12” to refer to mode pair 1 and 2, consistent with the subscript notation used in  $\beta_{mn}$ . As the range increases, the RDCs progressively fade—starting at lower frequencies—indicating significant attenuation of the third mode at an early stage (Fig. 1 (b) and (c)). In contrast, the first mode pair 12 remains persistent throughout the entire scenario (up to 19:45). The interference pattern of this mode pair enabled range estimation up to 45 km using a single constant WI.

**Estimated WI:** To ensure consistency with the range estimation analysis in the main manuscript, we estimate a single WI value using the spectrogram spanning 18:58 to 19:45, assuming that the waveguide invariant

associated with mode pair 12 remains stable over this duration. As shown in Fig. 1(b), mode pair 12 becomes dominant beginning around 19:03. Extending the window back to 18:58 allowed for additional data points and alignment with the time frame used in the main analysis, though mode pairs 13 and 23 still contribute to the earlier portion of the spectrogram. Ideally, using shorter spectrograms would enable assessment of temporal variability in the WI. However, accurate pairwise WI estimation is limited by resolution constraints, and longer spectrograms are required to achieve sufficient slope resolution in the Radon domain.

Using the normalized Radon transform, we estimate the WI of mode pair 12 to be 1.12, as shown in Fig. 2 (a), where each candidate WI corresponds to a hypothetical slope of the RDCs. Since only one prominent RDC corresponding to mode pair 12 persists in the 18:58–19:45 interval,  $\beta_{12}$  effectively represents the scalar WI of the environment. The corresponding RDC is displayed in Fig. 2 (b). In contrast, the WI value of 1.18 reported in the main manuscript was computed using a shorter spectrogram (18:58–19:10), where multiple mode pairs were active. Manual measurements of RDC slopes for different mode pairs during that interval yielded values between 1.11 and 1.20, suggesting modest variability. Moreover, resolution analysis shows that using a 47-minute spectrogram yields an estimated WI uncertainty of approximately  $\pm 0.15$ , while a 10-minute spectrogram would result in significantly higher uncertainty due to coarse resolution in the  $\log(\Delta k)$  domain. This estimated uncertainty reflects only the limits imposed by resolution and does not account for additional sources of error such as background noise, model mismatch, or temporal variability. These findings support the use of a longer spectrogram and indicate that the WI value of 1.18 reported in

the main manuscript lies within the expected uncertainty bounds of the mode-pairwise WI estimate derived here.

There are multiple sources of error in the current computation. Notably, we made the assumption of constant geoacoustic properties (such as SSP and seabed characteristics) over the 47-minute period. The intensities at each frequency were normalized by their maximum value, but acoustic intensities at broadband-only frequencies are expected to have lower SNR. Additionally, the mode pairwise WI values may vary across frequency bins<sup>5</sup>, and the values observed here are interpreted as averages of these variations. Furthermore, errors may arise from linear interpolation performed to obtain the data in the logarithmic domain.

### III. CONCLUSION

This study demonstrated the feasibility of characterizing the shallow-water acoustic environment using mode-pairwise WI analysis. By examining the RDCs derived from shorter spectrograms, we identified a dominant mode pair that persisted beyond 19:08, allowing the estimation of a single WI value of 1.12. The analysis revealed that attenuation reduced the number of propagating modes at longer ranges, leaving only the first mode pair for reliable range estimation up to 45 km. Despite the challenges of limited modal diversity and potential variability in geoacoustic properties, the estimated WI value of  $\beta = 1.18$  reported in the main manuscript lies within the uncertainty range of the WI value obtained via mode-pairwise analysis.

<sup>1</sup>G. Byun and H. C. Song, "The waveguide invariant for a Pekeris waveguide," *J. Acoust. Soc. Am.* **151**(2), 846–851 (2022).

<sup>2</sup>Y.-M. Jiang, C. W. Holland, S. E. Dosso, and J. Dettmer, "Depth and frequency dependence of geoacoustic properties on the New England Mud Patch from reflection coefficient inversion," *J. Acoust. Soc. Am.* **154**(4), 2383–2397 (2023).

<sup>3</sup>M. S. Ballard, D. D. Garcia, K. M. Lee, G. R. Venegas, A. R. McNeese, P. S. Wilson, and J. D. Chaytor, "Direct measurements of sediment geoacoustic properties in the New England Mud Patch and shelf break," *J. Acoust. Soc. Am.* **156**(4), 2889–2902 (2024).

<sup>4</sup>D. Rouseff and R. C. Spindel, "Modeling the waveguide invariant as a distribution," *AIP Conf. Proc.* **621**(1), 137–150 (2002).

<sup>5</sup>Y. Le Gall and J. Bonnel, "Separation of moving ship striation patterns using physics-based filtering," *Proceedings of Meetings on Acoustics* **19**(1), 070073 (2013).

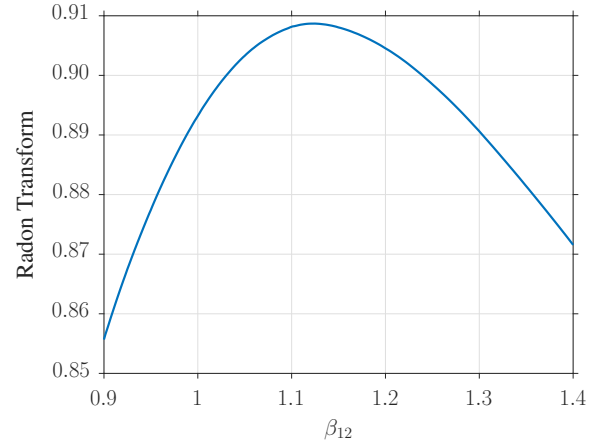

(a)

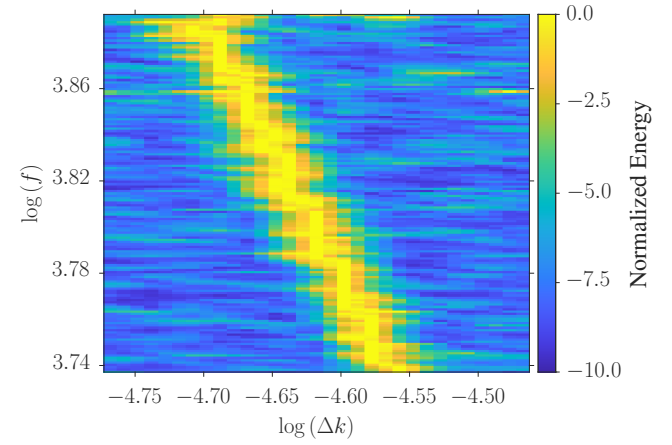

(b)

FIG. 2. (a) Radon transform output as a function of hypothetical mode pairwise WI values ( $\beta_{12}$ ), showing the maximum response at  $\beta = 1.12$ , indicating the dominant mode pair's WI value. The normalized Radon transform curve demonstrates the systematic estimation of the WI using the log-log domain of  $\Delta k$  and  $f$ . (b) Logarithmic plot of relative dispersion curves (RDCs) for mode pair 12, depicting the slope of the RDC in the log-log domain. The slope is directly related to the WI of the mode pair, obtained from acoustic recordings between 18:58 and 19:45.
